# Supplementary material for: Functional effects of schizophrenia-linked genetic variants on intrinsic single-neuron excitability: A modeling study
Source: arXiv:1509.07258 source file (2015-09-24)
Supplement: Supplementary file 1 [file supplementary.pdf]

Functional effects of schizophrenia-linked genetic variants on intrinsic single-neuron excitability: A modeling study. Supplemental information

# Methods

## The L5PC model

The current balance equation for each compartment of the neuron can be written as

$$C_m \frac{\partial V}{\partial t} = I_{Nat} + I_{Nap} + I_h + I_m + I_{Kp} + I_{Kt} + I_{Kv3.1} + I_{CaHVA} + I_{CaLVA} + I_{SK} + I_l + I_{axial},$$

where each type of current, except for the axial current, can be described as a multiplication of activation and inactivation variables as

$$I = \bar{g} m^{N_m} h^{N_h} (E - V).$$

Here, $\bar{g}$ is the maximal conductance of the ion channels, $m$ and $h$ are the activation and inactivation variables while $N_m$ and $N_h$ are constants describing their sensitivities, and $E$ is the reversal potential corresponding to the ionic species. Reversal potentials of $Na^+$ and $K^+$ are constants ($E_{Na} = 50$ mV, $E_K = -85$ mV), while the reversal potential of $Ca^{2+}$ depends on the intracellular [$Ca^{2+}$]: $E_{Ca}$ varied between 96 mV and 120 mV in our simulations. The dynamics of the activation and inactivation variables are defined as

$$\frac{dm}{dt} = \frac{m - m_\infty}{\tau_m} \quad \text{and} \quad \frac{dh}{dt} = \frac{h - h_\infty}{\tau_h},$$

where $m_\infty$, $h_\infty$, $\tau_m$, and $\tau_h$ are functions of membrane potential $V$. Typically, functions $m_\infty$ and $h_\infty$ have a sigmoidal shape, where the half-activation and half-inactivation voltages are determined by one or more (depending on ion channel) parameters each. We denotate these parameters $V_{\mathrm{offm}*}$ and $V_{\mathrm{offh}*}$, where $*$ stands for further specifications if there are multiple parameters affecting the half-(in)activation voltage. In a similar fashion, parameters $V_{\mathrm{slom}*}$ and $V_{\mathrm{sloh}*}$ affect the slopes of the (in)activation curves, and parameters $\tau_{\mathrm{m}*}$ and $\tau_{\mathrm{offh}*}$ influence the time constants. As an exception, the activation of $I_{SK}$ is solely dependent on the intracellular [$Ca^{2+}$], and this dependence is quantified by half-activation concentration parameter $c_{\mathrm{off}}$ and slope parameter $c_{\mathrm{slo}}$. The intracellular [$Ca^{2+}$] obeys the following dynamics:

$$\frac{d[\mathrm{Ca}^{2+}]_i}{dt} = \frac{I_{CaHVA} + I_{CaLVA}}{2\gamma F d} - \frac{[\mathrm{Ca}^{2+}]_i - c_{\min}}{\tau_{\mathrm{decay}}},$$

where $I_{CaHVA}$ and $I_{CaLVA}$ are the high and low-voltage activated $Ca^{2+}$ currents entering the considered cell segment, $\gamma$ represents the fraction of $Ca^{2+}$ ions entering the cell that contribute to the intracellular [$Ca^{2+}$], $F$ the Faraday constant, $d$ is the depth of the sub-membrane layer considered for calculation of concentration, $c_{\min}$ the resting intracellular [$Ca^{2+}$], and $\tau_{\mathrm{decay}}$ is the decay time constant of the intracellular [$Ca^{2+}$]. The simulation codes are provided in the ModelDB entry 169457 (https://senselab.med.yale.edu/ModelDB).

## Channel activation and inactivation dynamics

Here, the model equations and parameter values are listed for all ion channels. The maximal conductances $\bar{g}$ are different for different parts of the neuron: The subindex $s$ refers to soma, $ad$ to apical dendrite, $bd$ to basal dendrite, and $ax$ to axon, and for each current type all unshown maximal conductances are zero. For the non-specific ionic currents and $Ca^{2+}$ currents, the maximal conductances vary spatially along the apical dendrite in the following way. In the "hot zone", which lies on the distance 650µm–850µm, the maximal conductances of $Ca^{2+}$ currents are ten or hundredfold larger than elsewhere in the apical dendrite. The maximal conductances of the non-specific ionic current in turn grow exponentially from 0 to the length of the longest branch, $L_{\max}$, which is 1300 µm in this study. The numerical values correspond to the control neuron values and may be varied in the variant neurons.

### Fast inactivating $Na^+$ current, $I_{Nat}$

$$\alpha_m = -\frac{1}{\tau_{\mathrm{ma}}} \cdot \frac{V_{\mathrm{offm}} - V}{1 - \exp(\frac{(V_{\mathrm{offm}} - V)}{V_{\mathrm{slom}}})}$$

$$\beta_m = \frac{1}{\tau_{\text{mb}}} \cdot \frac{V_{\text{offm}} - V}{1 - \exp(\frac{-(V_{\text{offm}} - V)}{V_{\text{slom}}})}$$

$$\alpha_h = \frac{1}{\tau_{\text{ha}}} \cdot \frac{V_{\text{offh}} - V}{1 - \exp(\frac{(V_{\text{offh}} - V)}{V_{\text{sloh}}})}$$

$$\beta_h = -\frac{1}{\tau_{\text{hb}}} \cdot \frac{V_{\text{offh}} - V}{1 - \exp(\frac{-(V_{\text{offh}} - V)}{V_{\text{sloh}}})}$$

$$m_\infty = \frac{\alpha_m}{\alpha_m + \beta_m}$$

$$h_\infty = \frac{\alpha_h}{\alpha_h + \beta_h}$$

$$\tau_m = \frac{1}{T_{\text{adj}}(\alpha_m + \beta_m)}$$

$$\tau_h = \frac{1}{T_{\text{adj}}(\alpha_h + \beta_h)}$$

$V_{\text{offm}} = -38$ mV, $V_{\text{offh}} = -66$ mV, $V_{\text{slom}} = 6.0$ mV, $V_{\text{sloh}} = 6.0$ mV, $\tau_{\text{ma}} = 5.49$ ms, $\tau_{\text{mb}} = 8.06$ ms, $\tau_{\text{ha}} = 66.67$ ms, $\tau_{\text{hb}} = 66.67$ ms, $\bar{g}_s = 2.04$ S/cm$^2$, $\bar{g}_{ad} = 0.0213$ S/cm$^2$, $N_m = 3$, $N_h = 1$

**Persistent Na$^+$ current,** $I_{Nap}$

$$m_\infty = \frac{1}{1 + \exp(\frac{V_{\text{offm}} - V}{V_{\text{slom}}})}$$

$$h_\infty = \frac{1}{1 + \exp(-\frac{V_{\text{offh}} - V}{V_{\text{sloh}}})}$$

$$\alpha_m = -\frac{1}{\tau_{\text{ma}}} \cdot \frac{V_{\text{offma}} - V}{1 - \exp(\frac{(V_{\text{offma}} - V)}{V_{\text{sloma}}})}$$

$$\beta_m = \frac{1}{\tau_{\text{mb}}} \cdot \frac{V_{\text{offmb}} - V}{1 - \exp(\frac{-(V_{\text{offmb}} - V)}{V_{\text{slomb}}})}$$

$$\alpha_h = \frac{1}{\tau_{\text{ha}}} \cdot \frac{V_{\text{offha}} - V}{1 - \exp(-\frac{V_{\text{offha}} - V}{V_{\text{sloha}}})}$$

$$\beta_h = -\frac{1}{\tau_{\text{hb}}} \cdot \frac{V_{\text{offhb}} - V}{1 - \exp(\frac{V_{\text{offhb}} - V}{V_{\text{slohb}}})}$$

$$\tau_m = \frac{6}{T_{\text{adj}}(\alpha_m + \beta_m)}$$

$$\tau_h = \frac{1}{T_{\text{adj}}(\alpha_h + \beta_h)}$$

$V_{\text{offm}} = -52.6$ mV, $V_{\text{slom}} = 4.6$ mV, $V_{\text{offma}} = -38$ mV, $V_{\text{offmb}} = -38$ mV, $V_{\text{sloma}} = 6.0$ mV, $V_{\text{slomb}} = 6.0$ mV, $\tau_{\text{ma}} = 5.49$ ms, $\tau_{\text{mb}} = 8.06$ ms, $V_{\text{offh}} = -48.8$ mV, $V_{\text{sloh}} = 10.0$ mV, $V_{\text{offha}} = -17$ mV, $V_{\text{offhb}} = -64.4$ mV, $V_{\text{sloha}} = 4.63$ mV, $V_{\text{slohb}} = 2.63$ mV, $\tau_{\text{ha}} = 347222.2$ ms, $\tau_{\text{hb}} = 144092.2$ ms, $\bar{g}_s = 0.00172$ S/cm$^2$, $N_m = 3$, $N_h = 1$

**Non-specific cation current,** $I_h$

$$\alpha_m = -\frac{1}{\tau_{\text{ma}}} \cdot \frac{V_{\text{offma}} - V}{\exp(-\frac{V_{\text{offma}} - V}{V_{\text{sloma}}}) - 1}$$

$$\beta_m = \frac{1}{\tau_{\text{mb}}} \exp(-\frac{V_{\text{offmb}} - V}{V_{\text{slomb}}})$$

$$m_\infty = \frac{\alpha_m}{\alpha_m + \beta_m}$$

$$\tau_m = \frac{1}{\alpha_m + \beta_m}$$

$E = -45.0$ mV, $V_{\text{offma}} = -154.9$ mV, $V_{\text{sloma}} = 11.9$ mV, $\tau_{\text{ma}} = 155.52$ ms, $V_{\text{offmb}} = 0.0$ mV, $V_{\text{slomb}} = 33.1$ mV, $\tau_{\text{mb}} = 5.18$ ms, $\bar{g}_s = 0.0002$ S/cm$^2$, $\bar{g}_{ad} = -0.00017392$ S/cm$^2 + 0.0004174$ S/cm$^2 \cdot \exp(3.6161x/L_{\text{max}})$, $\bar{g}_{bd} = 0.0002$ S/cm$^2$, $N_m = 1$, $N_h = 0$

**Muscarinic K$^+$ current, $I_m$**

$$\alpha_m = \frac{1}{\tau_{\text{ma}}} \exp(-\frac{V_{\text{offma}} - V}{V_{\text{sloma}}})$$
$$\beta_m = \frac{1}{\tau_{\text{mb}}} \exp(\frac{V_{\text{offmb}} - V}{V_{\text{slomb}}})$$
$$m_\infty = \frac{\alpha_m}{\alpha_m + \beta_m}$$
$$\tau_m = \frac{1}{T_{\text{adj}}(\alpha_m + \beta_m)}$$

$V_{\text{offma}} = -35$ mV, $V_{\text{sloma}} = 10$ mV, $\tau_{\text{ma}} = 303.03$ ms, $V_{\text{offmb}} = -35$ mV, $V_{\text{slomb}} = 10$ mV, $\tau_{\text{mb}} = 303.03$ ms, $\bar{g}_{ad} = 0.0000675$ S/cm$^2$, $N_m = 1$, $N_h = 0$

**Slow inactivating K$^+$ current, $I_{Kp}$**

$$m_\infty = \frac{1}{1 + \exp(\frac{V_{\text{offm}} - V}{V_{\text{slom}}})}$$
$$h_\infty = \frac{1}{1 + \exp(-\frac{V_{\text{offh}} - V}{V_{\text{sloh}}})}$$
$$\tau_m = \begin{cases} \frac{\tau_{\text{mmin}} + \tau_{\text{mdiff1}} \exp(-\frac{V_{\text{offmt}} - V}{V_{\text{slomt}}})}{T_{\text{adj}}}, & \text{if } V \leq V_{thresh} \\ \frac{\tau_{\text{mmin}} + \tau_{\text{mdiff2}} \exp(\frac{V_{\text{offmt}} - V}{V_{\text{slomt}}})}{T_{\text{adj}}}, & \text{if } V > V_{thresh} \end{cases}$$
$$\tau_h = \frac{\tau_{\text{hmin}} + (\tau_{\text{hdiff1}} - \tau_{\text{hdiff2}}(V_{\text{offht1}} - V)) \exp\left(-\left(\frac{V_{\text{offht2}} - V}{V_{\text{sloht}}}\right)^2\right)}{T_{\text{adj}}}$$
$$V_{thresh} = V_{\text{offmt}} - \frac{V_{\text{slomt}}}{2} \log\left(\frac{\tau_{\text{mdiff1}}}{\tau_{\text{mdiff2}}}\right)$$

$V_{\text{offm}} = -11$ mV, $V_{\text{slom}} = 12$ mV, $V_{\text{offmt}} = -10$ mV, $V_{\text{slomt}} = 38.46$ mV, $\tau_{\text{mmin}} = 1.25$ ms, $\tau_{\text{mdiff1}} = 175.03$ ms, $\tau_{\text{mdiff2}} = 13$ ms, $V_{\text{offh}} = -64$ mV, $V_{\text{sloh}} = 11$ mV, $V_{\text{offht1}} = -65$ mV, $V_{\text{offht2}} = -85$ mV, $V_{\text{sloht}} = 48$ mV, $\tau_{\text{hmin}} = 360$ ms, $\tau_{\text{hdiff1}} = 1010$ ms, $\tau_{\text{hdiff2}} = 24$ ms/mV, $\bar{g}_s = 0.00223$ S/cm$^2$, $N_m = 2$, $N_h = 1$

**Fast inactivating K$^+$ current, $I_{Kt}$**

$$m_\infty = \frac{1}{1 + \exp(\frac{V_{\text{offm}} - V}{V_{\text{slom}}})}$$
$$h_\infty = \frac{1}{1 + \exp(-\frac{V_{\text{offh}} - V}{V_{\text{sloh}}})}$$
$$\tau_m = \frac{\tau_{\text{mmin}} + \tau_{\text{mdiff}} \exp\left(-\left(\frac{V_{\text{offmt}} - V}{V_{\text{slomt}}}\right)^2\right)}{T_{\text{adj}}}$$
$$\tau_h = \frac{\tau_{\text{hmin}} + \tau_{\text{hdiff}} \exp\left(-\left(\frac{V_{\text{offht}} - V}{V_{\text{sloht}}}\right)^2\right)}{T_{\text{adj}}}$$

$V_{\text{offm}} = -10$ mV, $V_{\text{slom}} = 19$ mV, $V_{\text{offh}} = -76$ mV, $V_{\text{sloh}} = 10$ mV, $V_{\text{offmt}} = -81$ mV, $V_{\text{slomt}} = 59$ mV, $\tau_{\text{mmin}} = 0.34$ ms, $\tau_{\text{mdiff}} = 0.92$ ms, $V_{\text{offht}} = -83$ mV, $V_{\text{sloht}} = 23$ mV, $\tau_{\text{hmin}} = 8$ ms, $\tau_{\text{hdiff}} = 49$ ms, $\bar{g}_s = 0.0812$ S/cm$^2$, $N_m = 4$, $N_h = 1$

**Fast, non inactivating K$^+$ current, $I_{Kv3.1}$**

$$m_\infty = \frac{1}{1 + \exp(\frac{V_{\text{offm}} - V}{V_{\text{slom}}})}$$
$$h_\infty = \frac{1}{T_{\text{adj}}\left(1 + \exp(\frac{V_{\text{offh}} - V}{V_{\text{sloh}}})\right)}$$

$V_{\text{offma}} = 18.7$ mV, $V_{\text{offmt}} = -46.56$ mV, $V_{\text{sloma}} = 9.7$ mV, $V_{\text{slomt}} = 44.14$ mV, $\tau_{\text{mmax}} = 4.0$ ms, $\bar{g}_s = 0.693$ S/cm$^2$, $\bar{g}_{ad} = 0.000261$ S/cm$^2$, $N_m = 1$, $N_h = 0$

**High-voltage-activated $Ca^{2+}$ current, $I_{CaHVA}$**

$$\alpha_m = -\frac{1}{\tau_{\text{ma}}} \cdot \frac{V_{\text{offma}} - V}{1 - \exp(\frac{V_{\text{offma}} - V}{V_{\text{sloma}}})}$$

$$\beta_m = \frac{1}{\tau_{\text{mb}}} \exp(-\frac{V_{\text{offmb}} - V}{V_{\text{slomb}}})$$

$$m_\infty = \frac{\alpha_m}{\alpha_m + \beta_m}$$

$$\tau_m = \frac{1}{\alpha_m + \beta_m}$$

$$\alpha_h = \frac{1}{\tau_{\text{ha}}} \exp(\frac{V_{\text{offha}} - V}{V_{\text{sloha}}})$$

$$\beta_h = -\frac{1}{\tau_{\text{hb}}} \cdot \frac{1}{1 + \exp(\frac{(V_{\text{offhb}} - V)}{V_{\text{slohb}}})}$$

$$h_\infty = \frac{\alpha_h}{\alpha_h + \beta_h}$$

$$\tau_h = \frac{1}{\alpha_h + \beta_h}$$

$V_{\text{offma}} = -27$ mV, $V_{\text{offmb}} = -75$ mV, $V_{\text{offha}} = -13$ mV, $V_{\text{offhb}} = -15$ mV, $V_{\text{sloma}} = 3.8$ mV, $V_{\text{slomb}} = 17$ mV, $V_{\text{sloha}} = 50$ mV, $V_{\text{slohb}} = 28$ mV, $\tau_{\text{ma}} = 18.18$ ms, $\tau_{\text{mb}} = 1.06$ ms, $\tau_{\text{ha}} = 2188.18$ ms, $\tau_{\text{hb}} = 153.85$ ms, $\bar{g}_s = 0.000992$ S/cm$^2$, $\bar{g}_{ad,\text{hot}} = 0.000555$ S/cm$^2$, $\bar{g}_{ad} = 0.0000555$ S/cm$^2$, $N_m = 2$, $N_h = 1$

**Low-voltage-activated $Ca^{2+}$ current, $I_{CaLVA}$**

$$m_\infty = \frac{1}{1 + \exp(\frac{V_{\text{offm}} - V}{V_{\text{slom}}})}$$

$$h_\infty = \frac{1}{1 + \exp(-\frac{V_{\text{offh}} - V}{V_{\text{sloh}}})}$$

$$\tau_m = \tau_{\text{mmin}} + \frac{\tau_{\text{mdiff}}}{T_{\text{adj}} \left(1 + \exp(-\frac{V_{\text{offmt}} - V}{V_{\text{slomt}}})\right)}$$

$$\tau_h = \tau_{\text{hmin}} + \frac{\tau_{\text{hdiff}}}{T_{\text{adj}} \left(1 + \exp(-\frac{V_{\text{offht}} - V}{V_{\text{sloht}}})\right)}$$

$V_{\text{offma}} = -40.0$ mV, $V_{\text{offmt}} = -35.0$ mV, $V_{\text{offha}} = -90.0$ mV, $V_{\text{offht}} = -50.0$ mV, $V_{\text{sloma}} = 6.0$ mV, $V_{\text{slomt}} = 5.0$ mV, $V_{\text{sloha}} = 6.4$ mV, $V_{\text{sloht}} = 7.0$ mV, $\tau_{\text{mmin}} = 5.0$ ms, $\tau_{\text{mdiff}} = 20.0$ ms, $\tau_{\text{hmin}} = 20.0$ ms, $\tau_{\text{hdiff}} = 50.0$ ms, $\bar{g}_s = 0.00343$ S/cm$^2$, $\bar{g}_{ad,\text{hot}} = 0.0187$ S/cm$^2$, $\bar{g}_{ad} = 0.000187$ S/cm$^2$, $N_m = 2$, $N_h = 1$

**Small-conductance $Ca^{2+}$-activated $K^+$ current, $I_{SK}$**

$$m_\infty = \frac{1}{1 + \left(\frac{[\text{Ca}^{2+}]_i}{c_{\text{off}}}\right)^{-c_{\text{slo}}}}$$

$c_{\text{off}} = 0.00043$ mM, $c_{\text{slo}} = 4.8$, $\bar{g}_s = 0.0441$ S/cm$^2$, $\bar{g}_{ad} = 0.0012$ S/cm$^2$, $N_m = 1$, $N_h = 1$

**Leak current, $I_{leak}$**
$E = -90$ mV, $\bar{g}_s = 0.0000338$ S/cm$^2$, $\bar{g}_{ad} = 0.0000589$ S/cm$^2$, $\bar{g}_{bd} = 0.0000467$ S/cm$^2$, $N_m = 0$, $N_h = 0$

**Intracellular [$Ca^{2+}$] dynamics**

$$\frac{d[\text{Ca}^{2+}]_i}{dt} = \frac{I_{CaHVA} + I_{CaLVA}}{2\gamma F d} - \frac{[\text{Ca}^{2+}]_i - c_{\text{min}}}{\tau_{\text{decay}}}$$

$\gamma = 0.05$, $\tau_{\text{decay}} = 80$ ms, $d = 0.1$ µm, $c_{\text{min}} = 10^{-4}$ mM

**Temperature adjustment factor**

$$T_{\text{adj}} = 2.3^{\frac{34-21}{10}}$$

## Functional genomics literature review

Many of the genes that are now confirmed to be linked to SCZ, have previously been shown to play a role in regulating the activation/inactivation kinetics of certain types of cellular transmembrane currents in animal or *in vitro* studies. Typically, these studies involved transfection of ion channel-encoding DNA into cells that normally do not express the considered ion channels, and documentation on how a variant DNA changed the electrophysiological properties of the cells compared to the cells transfected with control DNA. Moreover, many studies have demonstrated the effects of certain variants of a calcium signaling toolkit gene [S1] on the dynamics of the $Ca^{2+}$ concentration in the intracellular medium.

We searched through the literature on functional genomics for genes *CACNA1C*, *CACNB2*, *CACNA1I*, *ATP2A2*, *HCN1*, *CACNA1D*, *CACNA1S*, *SCN1A*, *SCN7A*, *SCN9A*, *KCNN3*, *KCNS3*, *KCNB1*, *KCNG2*, *KCNH7*, and *ATP2B2* to find data on how genetic variations change the ion channel behavior or intracellular $Ca^{2+}$ dynamics. Due to shortness of data reported for a single animal and cell type, we included studies performed in various animal species and across different tissues. We concentrated on studies that fulfilled the following conditions:

- The study applied a genetic variant of one of the genes of interest and the gene is likely to be expressed in L5PCs.
- The properties of the cell expressing the gene variant were studied using electrophysiology or $Ca^{2+}$ imaging.
- The deviation between the variant cell property and the control cell property could be implemented in the applied neuron model [S2] as a change of a model parameter value.
- The observed effect of the gene variant was not solely on the expression or ion channel density level.

The last condition, which ruled out studies where the effect was only shown on channel density, was set due to the multitude of pathways that may contribute to such an effect [S3]. By contrast, the effects on channel kinetics (activation and inactivation threshold potentials, sensitivity to membrane potential, and opening/closing time constants) were expected to be more straightforwardly dependent on the way these channels are genetically coded. However, data on differences in ion channel expression bear an important aspect of the total ionic behavior as well, and should therefore be introduced in the future, although compensatory mechanisms may contribute to cancel the effects of changes in expression *in vivo* (cf. [S4]).

Table 1 shows all studies that were found to obey the above conditions. An expansion of this table is given in Table S1, added with details about the effects of each variant and the underlying experimental data. The six first genes of Table 1 belong to the calcium signaling toolkit. The genes *CACNA1C*, *CACNB2*, and *CACNA1D*, encode $\alpha$ or $\beta$ subunits of HVA $Ca^{2+}$ channels, and *CACNA1I* gene encodes an $\alpha$ subunit of an LVA $Ca^{2+}$ channel. Genes *ATP2A2* and *ATP2B2* encode intracellular $Ca^{2+}$ transporters, namely sarco/endoplasmic reticulum $Ca^{2+}$ ATPase (SERCA) and plasma membrane $Ca^{2+}$ ATPase (PMCA). The rest of the listed genes encode ion channels of other ionic species. *SCN1A* and *SCN9A* encode $\alpha$ subunits of $Na^+$ channels, which we considered to contribute to the currents $I_{Nat}$ and $I_{Nap}$ in the neuron model. *KCNB1* encodes a subunit that contributes to the slow, delayed rectifier $K^+$ current in L5PCs [S5, S6], which is denoted by $I_{Kp}$ in the neuron model. *KCNS3* encodes an electrically silent subunit, which yet together with the subunit encoded by *KCNB1* forms slowly inactivating $K^+$ channels [S5, S7]: these channels contribute to the current $I_{Kp}$ as well. *KCNN3* encodes a subunit for a $Ca^{2+}$-activated small-conductance $K^+$ channel (contributing to $I_{SK}$), and *HCN1* encodes a subunit for a non-specific ion channel (contributing to $I_h$). Not all of these genes have been shown to be expressed in thick-tufted L5PCs in specific, however, we confirmed in Allen Brain Atlas (mouse) and Human Protein Atlas that they all show expression in the cortex. Certain studies on *CACNA1S* fulfilled all other above conditions, but the gene is not expressed anywhere in the brain, and therefore we disregarded them.

Some of the studies cited in Table 1 considered several variant types, and in these cases, the range of possible effects on model parameters is considered (see Table S1). If the range spanned both increasing and decreasing effects, the analyses were carried out for both end points of the range, otherwise only the maximal deviation from the control value was considered. Also, in case one of the end points of the range was very close to the control value, namely, at a distance less than 1 mV or less than 10% of the distance between control value and the other end point, only the endpoint with the larger deviation was considered.

The applied model of an L5PC is relatively abundant in biological detail, yet it groups together many different types of currents under one model current. This represents a hindrance to carrying out detailed computational studies on the contribution of different genes to neuron firing behavior. As for our study, for this reason we could not make a distinction between the contributions of L, N-, P-, and Q-type channels (HVA $Ca^{2+}$ current channels) to the activation of the SK current, which have been experimentally studied in e.g. [S8]. Taking into account this particular distinction would be an important extension to our modeling framework, as many of the SCZ-related $Ca^{2+}$ channel-encoding genes specifically encode L-type channel subunits (*CACNA1C*, *CACNA1D*, *CACNA1S*, *CACNB2*). Nevertheless, currently there are no L5PC models that would allow this.

## Scaling of gene variants

Due to the polygenic nature of SCZ, it has been proposed that none of the SCZ-related SNPs can alone cause the disorder, and that the disease may only be induced when sufficiently many of them are represented. This paradigm was adopted into the computational study at hand as follows. We first identified the parameter changes in the L5PC model [S2] that corresponded to the effects of a certain genetic variant. We then ran simulations on the neuron model, exploring the effects of one variant separately on the neuron's response to selected stimuli. If the variant altered the neural response dramatically, the genetic effect was scaled down (i.e. parameters were brought closer to the control values), so that there were no large

discrepancies between the control neuron and the mutant with the downscaled variant. The criteria for the downscaling were that no variant should alone change the number of action potentials to chosen stimuli or radically change the steady-state firing behavior of the neuron (control neuron referring to the model neuron exactly as described in [S2]). This approach was used in order to simulate the SCZ-related SNP effects, many of which are known to be subtle (cf. [S9]) in contrast to the large phenotypic effects caused by the variants of Table 1.

To scale down the effects of the variants of Table S1, the following procedure was applied. Firstly, a "standard spiking behavior" was defined as a firing behavior that fulfils the following five conditions:

**(I)** Exactly 4 spikes should be induced as a response to somatic square-current injection of 0.696 nA x 150 ms,

**(II)** Exactly 1 spike should be induced as a response to a distal (620 μm from soma) alpha-shaped synaptic conductance (time constant 5 ms, max. amplitude 0.0612 μS),

**(III)** Exactly 2 spikes should be induced as a response to a combined stimulus of somatic square-current injection (1.137 nA x 10 ms) and distal synaptic conductance (time constant 5 ms, max. amplitude 0.100 μS, applied 5ms after the somatic pulse),

**(IV)** The integrated difference between the f-I curves of the considered neuron and the control neuron should not be more than 10% of the integral of the control neuron f-I curve, and

**(V)** The membrane potential limit cycle should not be too different from the control neuron limit cycle ($d_{cc}(lc_1, lc_2) \leq 600$, see the section below for details).

The above-mentioned amplitudes 0.696 nA, 0.0612 μS, and 1.137 nA were chosen such that the control neuron most stably produces the named numbers of spikes with the default parameters — most stably in the sense that an equal change in current amplitude on logarithmic scale is required in order to produce one spike more or to produce one spike less. The conditions I–III restrict the magnitudes of short-time responses of the neuron, while the conditions IV–V concern continuous, steady-state firing. Secondly, the spiking behavior of cells expressing the genetic variations listed in Table 1 under the same stimuli is simulated. In case one or more of the conditions I–V are violated, the effect is scaled down, all parameters in proportion, to a fraction $c < 1$ of the original effect where the violation is for the first time observed. These threshold effect factors $c$ are listed in Table 2 for each variant together with the corresponding parameter changes, and the six variants that were used in Figures 2–6 are highlighted. As we do not know how small a parameter change effect should be to correspond to a small SNP effect, we consider variants with different scalings where the threshold effect factor $c$ is multiplied with another factor $\epsilon < 1$. In this work, we consider the scaling factor values $\epsilon = \frac{1}{2}$ and $\frac{1}{4}$, and we also display the effects of the corresponding opposite variants $\epsilon = -\frac{1}{2}$ and $-\frac{1}{4}$.

For those unscaled variants that did not violate the conditions I–V, we sought for the threshold effect up to twice the original effect, i.e. $c < 2$. If the variant still obeyed conditions I–V, we considered the original variant the $\epsilon = \frac{1}{2}$ variant and applied other scalings with respect to this choice.

The model parameters affected by the variants include quantities of various roles and dimensions (mV, mM, ms, etc.), which calls for a careful consideration how to scale them properly. We chose to perform this such that those parameters that may receive both negative and positive values were scaled linearly, while the parameters that receive only positive values were scaled on the logarithmic scale. In practice, this means that the differences in offset and reverse potentials ($V_{\text{offm}*}$, $V_{\text{offh}*}$, $E_{\text{Ih}}$) between control and variant neuron were expressed as an additive term ($\pm x$ mV), and this term $x$ was multiplied by a factor $c \in [0, 1]$ in the downscaling procedure. By contrast, the differences in all the other model parameters ($V_{\text{offc}*}$, $V_{\text{slo}*}$, $\tau_*$, $c_*$, $\gamma_*$) between control and variant neuron were expressed as a multiplication ($\times x$), where the downscaling caused this coefficient $x$ to be exponentiated by the same factor $c$. This procedure permits a continuum of parameter changes in the range $c \in [0, 1]$ that is directly applicable to amplified ($c > 1$) parameter changes as well. As an example, consider the mid-point of activation of the slow inactivating $K^+$ channel, $V_{\text{offm,Kp}} = -11$ mV. One of the variants of KCNB1 gene (fifth in Table 2) shifted this value by +14 mV, which gives the new value $V'_{\text{offm,Kp}} = 3$ mV. In such a case, it is not possible scale the parameter logarithmically, as the factor $x = V'_{\text{offm,Kp}}/V_{\text{offm,Kp}}$ to be exponentiated is negative. As a contrary example, the same variant changes the time constants of activation, $\tau_{\text{m}*,\text{Kp}}$, by −61%. In principle, this effect could be scaled both logarithmically and linearly in the range $c \in [0, 1]$. However, if the unscaled variant does not cause a violation of conditions I–V, we would study the effects of an "upscaled" variant all the way until $c = 2$. This would not be possible using linear scaling, as we would have to decrease the time constants of activation by 122%, leading to negative time constants.

## A distance metric for membrane potential limit cycles

A membrane potential limit cycle can be described as a 1-dimensional manifold in the space $\mathcal{LC} = \mathcal{V} \times d\mathcal{V}$, where $\mathcal{V}$ is the space of possible values for membrane potentials and $d\mathcal{V}$ is the space of possible values for time derivatives of membrane potential. Due to the difference in units for $x$ and $y$ axis, there is no obvious metric for this space, but such can easily be constructed. We define a bijection $f : \mathcal{LC} \to \mathbb{R}^2$ as

$$f(V, dV) = \left( \frac{V}{1.0 \text{ mV}}, \frac{dV}{7.026 \text{ mV/ms}} \right),$$

where the constant 7.026 was chosen such that the control neuron limit cycle spans an equal range on $x$ and $y$ axes when the soma is given a DC of amplitude 1.0 nA. Now, a distance metric in $d : \mathcal{LC} \times \mathcal{LC}$ can be defined as

$$d(x, y) = ||f(x) - f(y)||_2,$$

where $|| \cdot ||_2$ is a Euclidean norm. Furthermore, the distance of a point $x \in \mathcal{LC}$ from a limit cycle $lc \subset \mathcal{LC}$ can be defined as

$$d_c(x, lc) = \min_{y \in lc} ||f(x) - f(y)||.$$

To evaluate the difference between two limit cycles $lc_1, lc_2 \subset \mathcal{LC}$, we define

$$d_{cc}(lc_1, lc_2) = \frac{1}{2}\int_{lc_1} d_c(x, lc_2)dx + \frac{1}{2}\int_{lc_2} d_c(x, lc_1)dx.$$

Using the average of the two integrals makes sure that no part of either limit cycle is ignored: If only integral over points of $lc_1$ was used, the limit cycle $lc_2$ could have any "extra" part, for example an unusually long and slow hyperpolarization period or minor suboscillations, that might largely be disregarded in the integration as there are always some other points in $lc_2$ that lie nearer to $lc_1$.

Table S1: **Table of genetic variants and their maximal effects on our neuron model parameters.** The first column of the table shows the gene whose variant is studied. The second column shows the model parameters that are affected by the variant, as the third column shows the size of the effect. The fourth column gives the PubMed index of the article, where the effects of the variant are measured. The fifth column names the type of variant used, while the sixth and seventh columns show the cell type in which the effects are measured and the animals species used in the study. The final column may give extra information. The variants are listed in the order of genes that they affect. Asterisks represent an identical change to a set of variables as follows (applicable to those variables that exist in the considered ion channel type): offm* refers to variables $V_{\mathrm{offm}}$, $V_{\mathrm{offma}}$ and $V_{\mathrm{offmb}}$; offh* refers to variables $V_{\mathrm{offh}}$, $V_{\mathrm{offha}}$ and $V_{\mathrm{offhb}}$; slom* refers to variables $V_{\mathrm{sloma}}$ and $V_{\mathrm{slomb}}$; sloh* refers to variables $V_{\mathrm{sloha}}$ and $V_{\mathrm{slohb}}$; taum* refers to variables $\tau_{\mathrm{ma}}$, $\tau_{\mathrm{mb}}$, $\tau_{\mathrm{mmin}}$, $\tau_{\mathrm{mdiff}}$, $\tau_{\mathrm{mdiff1}}$ and $\tau_{\mathrm{mdiff2}}$; tauh* refers to variables $\tau_{\mathrm{ha}}$, $\tau_{\mathrm{hb}}$, $\tau_{\mathrm{hmin}}$, $\tau_{\mathrm{hdiff}}$, $\tau_{\mathrm{hmean}}$, $\tau_{\mathrm{hdiff1}}$ and $\tau_{\mathrm{hdiff2}}$.

| Gene | Model parameter | Effect | Paper | Type of variant | Cell type | Animal | Notes |
|---|---|---|---|---|---|---|---|
| CACNA1C | offm*_CaHVA<br>offh*_CaHVA | -25.9..-1.4 mV<br>-27.0..-3.8 mV | pubmed/19265197 | L429T, L434T, S435T, S435A S435P | TSA201 | human | -These represent variant of the IS6 segment |
| CACNA1C | offm*_CaHVA<br>offh*_CaHVA | -37.3..-9.7 mV<br>-30.0..-11.8 mV | pubmed/19265197 | L779T, I781T, I781P | TSA201 | human | -These are variants of IIS6 segment. Double (IIS6+IS6) mutant seems to have additive effect |
| CACNB2 | offh*_CaHVA<br>sloh*_CaHVA | -5.2 mV<br>-31% | pubmed/19358333 | T11I-mutant | TSA201 | human | -Small changes shown in offma, offmb and tau ignored |
| CACNB2 | taum*_CaHVA | +70% | pubmed/7723731 | A1B2 vs A1 alone | HEK293 | human/mouse | |
| CACNB2 | offm*_CaHVA<br>offh*_CaHVA<br>taum*_CaHVA<br>tauh*_CaHVA | -4.9..+4.9mV<br>-5.1..+5.1mV<br>-40%..+68%<br>-40%..+66% | pubmed/19723630 | N1 vs N3 vs N4 vs N5 | HEK293 | human/mouse | -Changes to voltage-dependence of taus ignored. |
| CACNA1D | offm*_CaHVA<br>slom*_CaHVA<br>offh*_CaHVA<br>sloh*_CaHVA<br>tauh*_CaHVA | -10.9..-8.5mV<br>-27..-13%<br>-3.0..+3.5mV<br>-12..-19%<br>+25% | pubmed/21998309<br>pubmed/21998310 | 42A splices transfected (Alternative splicing at C-terminus) | TSA201/HEK293 | human | -The variants are expressed in human and mouse brains; hence, the effect of genetic variances could be of opposite sign with respect to control |
| CACNA1D | offm*_CaHVA<br>slom*_CaHVA<br>offh*_CaHVA<br>sloh*_CaHVA<br>tauh*_CaHVA | -10.6..+3.4mV<br>-20..+12%<br>-5.3..+1.2mV<br>-34..-8%<br>-28% | pubmed/21998309<br>pubmed/21998310 | 43S splices transfected (Alternative splicing at C-terminus) | TSA201/HEK293 | human | -The variants are expressed in human and mouse brains; hence, the effect of genetic variances could be of opposite sign with respect to control |
| CACNA1D | offm*_CaHVA<br>slom*_CaHVA<br>tauh*_CaHVA | +3.5..+6.6mV<br>-25..+19%<br>-50..+12% | pubmed/20951705<br>pubmed/21054386 | CaV1.3 (-/-) vs control | AV node cells/ chromaffin cells | mouse | -Some time constants compared between single tau fits (as double tau fits not always well fitted) |
| CACNA1I | offma_CaLVA<br>offha_CaLVA<br>taum*_CaLVA<br>tauh*_CaLVA | -0.2..+1.3mV<br>-0.5..+1.6mV<br>-13..+45%<br>-20..+8% | pubmed/15254077 | Alternative splicing of exons 9 and 33 | HEK293 | human | -Maximum of effects at -40 or 0 mV on kinetics considered<br>-Changes in slope minuscule |
| ATP2A2 | gamma_CaDyn | -30..-40% | pubmed/10970890 | Heter. null mutation | myocytes | mouse | -Compensating mechanisms exist that prevent larger effects |
| ATP2B2 | decay_CaDyn | +15..+113% | pubmed/22789621 | Heter. knockout | Purkinje cells | mouse | -Compensatory mechanisms exist that prevent larger effects |
| ATP2B2 | decay_CaDyn<br>minCai_CaDyn | +32..+50%<br>+40% | pubmed/21232211 | Homozyg. knockout | Purkinje cells | mouse | |
| ATP2B2 | decay_CaDyn | +53..+345% | pubmed/17234811 | G283S-,G293S-mutant | CHO cells | human/mouse | -+53% for G293S, +345% for G283S |
| SCN1A | offm_Nat<br>offh_Nat<br>slom_Nat<br>sloh_Nat | -0.3mV<br>+5.0mV<br>+15%<br>+23% | pubmed/18632931 | FHM mutation Q1489K | Neocortex (cultured) | human/rat | -Slow inactivation could not be studied in detail in neurons |
| SCN1A | offm_Nat<br>offh_Nat<br>slom_Nat<br>sloh_Nat | +2.8mV<br>+9.6mV<br>-1.6%<br>+4.2% | pubmed/17397047 | FHM mutation L1649Q | TSA201 | human | -Electrophysiology done with the corresponding mutation L1636Q in the homologous SCN5A gene due to instabilities in recomb. bacteria |
| SCN9A | offh*_Nap | +6.8mV | pubmed/22136189 | I228M NaV1.7 variant | HEK293 | human | -Differences in activation and fast inactivation not significant |
| SCN9A | offh*_Nap<br>sloh_Nap<br>offm_Nat<br>offh_Nat<br>sloh_Nat | +3.5mV<br>-45%<br>-7.1mV<br>+17.0mV<br>-31% | pubmed/18945915 | A1632E NaV1.7 mutation | HEK293 | human | -Slow inactivation interpreted as inactivation of persistent (Nap) current and fast inactivation as inactivation of transient (Nat) current |
| SCN9A | offm_Nat<br>offh_Nat | -9.1mV<br>+3.1mV | pubmed/16392115 | L858F NaV1.7 mutation | HEK293 | human | -Activation and inact. curves closer to Nat than Nap currents |
| SCN9A | offm_Nat<br>offh_Nat | -7.6mV<br>+4.3mV | pubmed/15958509 | F1449V NaV1.7 mutation | HEK293 | human | -Activation and inact. curves closer to Nat than Nap currents |
| KCNS3 | taum*_Kp<br>tauh*_Kp<br>sloh_Kp | 0..+100%<br>+50..+150%<br>-50% | pubmed/10484328 | hKv2.1-(G4S)3-hKv9 fusion inserted (or hKv9 inserted explicitly) | HEK293 | human | -Fits not carried out in the paper, approximate values used. |
| KCNB1 | offm_Kp<br>offh_Kp<br>slom_Kp<br>sloh_Kp<br>taum*_Kp<br>tauh*_Kp | +5mV<br>+3mV<br>+11%<br>-14%<br>-50%<br>-47% | pubmed/21455829 | T203K mutant | HEK293 | human/mouse | -Double mutations studied as well, but they are not included here |
| KCNB1 | offm_Kp<br>offh_Kp<br>slom_Kp<br>sloh_Kp<br>taum*_Kp | +1mV<br>-6mV<br>+22%<br>+0%<br>-11% | pubmed/21455829 | T203D mutant | HEK293 | human/mouse | |

| | | | | | | | |
|---|---|---|---|---|---|---|---|
| | tauh*_Kp | -13% | | | | | |
| KCNB1 | offm_Kp<br>offh_Kp<br>slom_Kp<br>sloh_Kp<br>taum*_Kp<br>tauh*_Kp | +6mV<br>-8mV<br>+33%<br>+0%<br>-50%<br>-13% | pubmed/21455829 | S347K mutant | HEK293 | human/mouse | |
| KCNB1 | offm_Kp<br>offh_Kp<br>slom_Kp<br>sloh_Kp<br>taum*_Kp<br>tauh*_Kp | -28mV<br>-27mV<br>+11%<br>-29%<br>+13%<br>+127% | pubmed/21455829 | S347D mutant | HEK293 | human/mouse | |
| KCNB1 | offm_Kp<br>offh_Kp<br>slom_Kp<br>sloh_Kp<br>taum*_Kp<br>tauh*_Kp | +14mV<br>-21mV<br>+100%<br>+0%<br>-61%<br>+20% | pubmed/21455829 | T203W mutant | HEK293 | human/mouse | |
| KCNB1 | offm_Kp<br>offh_Kp<br>slom_Kp<br>sloh_Kp<br>taum*_Kp<br>tauh*_Kp | -13mV<br>-13mV<br>+33%<br>-29%<br>-5%<br>+413% | pubmed/21455829 | S347W mutant | HEK293 | human/mouse | |
| KCNN3 | offc_SK<br>sloc_SK | -14%<br>+24% | pubmed/14978258 | hSK3_ex4 isoform | TSA | human | -Activation curve constructed a bit differently from Hay model |
| HCN1 | offm*_Ih<br>slom*_Ih | -2.1..-26.5mV<br>-12..-36% | pubmed/17185333 | D135W, D135H, D135N mutants | HEK293 | human/mouse | -Other mutations studied as well, but they change the Ih current too dramatically |

# Supplemental results

Here, we extended the analyses carried out for the variants of Figures 2–6 by considering additional variants. Figures S1 and S2 show a compilation of statistics related to Figures 3–6 for all variants of Table 2: Figure S1 illustrates the range of steady-state $Ca^{2+}$ concentration oscillation, while Figure S2 shows the mean firing rate across the DC amplitudes used in the f-I curves, the temporal sensitivities of the $Ca^{2+}$ spike during up and down states, and the time window for an efficient suppression of a second apical stimulus. In Figure S1, the results are additionally plotted for the unscaled variants for reference, while in Figure S2, only unscaled variants are considered. The results of Figure S2 for the positively scaled ($\epsilon = \frac{1}{2}$) variant are also summarized in Table S2. Except for genes *KCNS3* and *KCNB1*, variants of all genes showed a notable impact on some of these statistics.

Changes in intracellular [$Ca^{2+}$] may be functionally relevant for many neural processes. Intracellular [$Ca^{2+}$] plays an important role in the activation of various second messenger cascades, which control a variety of cellular processes [S4, S10–S13], but these aspects are out of the scope of the current work. A more immediate effect of intracellular [$Ca^{2+}$] is the activation of $Ca^{2+}$-dependent $K^+$ -currents, such as the small-conductance $K^+$ current ($I_{SK}$). This current was included in the L5PC-model, and it is affected by the *KCNN* gene family. In Figure 2, the effects of the *KCNN3* variant were undetectable. This was because $I_{SK}$ currents are large only when both intracellular [$Ca^{2+}$] and the membrane potential are elevated — although the currents only need high [$Ca^{2+}$] to be activated, they can be large only when the membrane potential is far enough from the $K^+$ reversal potential, which is relatively near to the membrane resting potential. The effects of the *KCNN3* variant could be detected when a more enduring stimulus than a brief somatic pulse was applied, as done in Figures 3–6: these effects can also be observed in Figures S1 and S2.

Most of the variants that gave positive shift in [$Ca^{2+}$](Figure S1), also resulted in reduced firing rates (Figure 3). There was a correlation coefficient of -0.70 between the maximal [$Ca^{2+}$] value in the limit cycle and the integral of the measured f-I curve. An exception to this trend was the *KCNN3* variant, where the threshold [$Ca^{2+}$] was lower (in the positively scaled variants) than in the control neuron, see Table 2. When stimulated with the DC of amplitude 1.2 nA (Figure 4), this lower threshold caused the SK current to be upheld for a longer time after the spike than in the control neuron. This caused a delay in the timing of the next spike, allowing the [$Ca^{2+}$] to drop to a lower value before the next spike, and hence the oscillation of the [$Ca^{2+}$] remained at an overall lower level than in the control neuron (data not shown).

## Combinations of variants may cause large alterations of neuron excitability

The effects of the variants on neuron excitability, as explored in Figures 2–6, were relatively small when the variants were studied in isolation (this was also the intention behind the downscaling process). However, combinations of variants of different genes may have additive effects on the neuron excitability. We investigated the effect that combinations of several of the variants could have. Figure S3 shows a selected example of how a combination of variants altered the neuron firing properties considered in Figures 2–6. Although this version of the model neuron consists of downscaled variants, the properties of neuron excitability were remarkably modified.

In Figure S3, the selection was based on the property of inhibiting the second apical stimulus as shown in Figure 6: We combined such downscaled variants that had a lower threshold curve than the control neuron, i.e., variants that made it easier for the second apical stimulus to induce a spike, however picking maximum one variant per gene. See Table 2 for this selection. Large impacts of the combination of variants could be seen in both $Ca^{2+}$ responses (Figure S3A-B, S3D), temporal profiles of $Ca^{2+}$ spike generation (Figure S3E), and naturally the inhibition of a second stimulus (Figure S3F). The change in gain (Figure S3E) was nevertheless minor: Although all variants of the combination caused an increase in gain when in isolation (except for the *CACNA1I* variant which had a minuscule effect and *KCNN3* variant which had an ambiguous effect), these increases in gain were in most cases caused by an overall decrease in $Ca^{2+}$ currents. These changes were compensated for by a decrease of threshold [$Ca^{2+}$] of the SK current that is characteristic of the *KCNN3* variant, and hence the resulting f-I curve was relatively close to that of the control neuron.

The effect of the combination of variants on the $Ca^{2+}$ spike generation in Figure S3E is notable. The sensitivity of the $Ca^{2+}$ spike magnitude to the ISI could serve as a coincidence detection mechanism of synaptic inputs projected to different parts of the L5PC and thus form an important element in cortical information processing. A widening of the region of ISIs that produce a large $Ca^{2+}$ spike could weaken the coincidence detection ability of the neuron [S14], while an extensive narrowing of the curve would limit the regime for [$Ca^{2+}$] spike generation [S15] and hence contribute with a lesser total excitability. In the up-state protocol, the combination of $\epsilon = \frac{1}{4}$ variants only produce minor $Ca^{2+}$ spikes, and their temporal ISI window is narrowed down, while the combination of $\epsilon = \frac{1}{2}$ variants does not produce a $Ca^{2+}$ spike at all with the considered stimuli.

Due to lack of data on the interplay between different variants of a single gene, we only implemented a maximum of one variant per gene when we simulated combinations of variants. There is, however, evidence that SNPs or other variants located in different parts of the same gene may have additive effects on the ion channel kinetics, as shown in the case of mutations in different parts of the *CACNA1C* gene [S16]. Hence, given detailed information on such effects in other genes as well, the predictive power of our method could still be improved by allowing more diverse combinations of the same set of variants.

## Robustness of the analyses

To study the robustness of our findings, we performed similar analyses in a neuron model using an alternative set of fitted model parameters. We implemented the alternative neuron model, “Model 1”, as given in the first column of Table S1 in [S2].

The scaling of the variants was redone in this neuron model, and the variant neuron behaviour was quantified in a similar manner as done for the primary fit. Figure S4 shows the compilation of results obtained from the alternative model. The results are qualitatively similar for the majority of the variants. The only observable exceptions are the 12th variant in the third group of *CACNB2* variants and the second variant in the second group of *CACNA1D* variants, which caused a large depression of the $Ca^{2+}$ spike in the up-state protocol of the primary neuron model, shown as a missing bar in Figure S2C. By contrast, the dendritic membrane potential response in the same variants of the alternative neuron model did exceed the set threshold, leading to an observed (but narrowed-down) temporal window in Figure S4C.

We further analyzed the robustness of our findings using the primary neuron model fit but in an alternative neuron morphology. We applied and downscaled our variants using the cell #2 morphology of [S2], and performed the same analyses as done with the primary neuron morphology, cell #1. The firing rates were in general smaller in cell #2: A somatic DC of amplitude 1.2 nA caused the control neuron to fire with a frequency of 15.4 Hz, whereas the corresponding rate in cell #1 was 16.9 Hz. The up- and down-state protocols did not produce responses directly comparable those of cell #1, and hence, we omitted these analyses in cell #2. By contrast, the property of inhibiting a second apical stimulus was preserved in cell #2, although in a slightly different regime. In cell #2, a nearly doubled maximal conductance w.r.t. that in cell #1 was required to make the neuron spike when the synaptic inputs were uniformly distributed along the apical dendrite ($g_{th}$ = 5.0 μS vs. 2.8 μS in cell #1). Accordingly, the ratio $c_g$ between the threshold conductance for eliciting a second spike and that for eliciting the first spike ($g_{th}$) was lower: In the control case of cell #2, the factor $c_g$ varied from 0.44 to 1.91, while the corresponding range in cell #1 was from 0.51 to 5.13. To compensate for this effect, we analyzed the PPI temporal window in terms of a lower threshold factor, namely, we measured the first and last ISI for which $c_g$ exceeded the value 1.5 (3.0 in cell #1).

The compilation of results obtained from simulations with cell #2 are shown in Figure S5. The amplitudes of variant effects are different than in cell #1 (see Figure S2), but the direction of the variant effects are the same as in cell #1.

# References


S1. MJ Berridge, P Lipp, and MD Bootman. “The versatility and universality of calcium signalling”. In: *Nature Rev Mol Cell Biol* 1.1 (2000), pp. 11–21.

S2. E Hay, S Hill, F Schürmann, H Markram, and I Segev. “Models of neocortical layer 5b pyramidal cells capturing a wide range of dendritic and perisomatic active properties”. In: *PLoS Comput Biol* 7 (2011), e1002107.

S3. B Rosati and D McKinnon. “Regulation of ion channel expression”. In: *Circ Res* 94.7 (2004), pp. 874–883.

S4. T O’Leary, AH Williams, A Franci, and E Marder. “Cell types, network homeostasis, and pathological compensation from a biologically plausible ion channel expression model”. In: *Neuron* 82.4 (2014), pp. 809–821.

S5. D Guan, T Tkatch, D Surmeier, W Armstrong, and R Foehring. “Kv2 subunits underlie slowly inactivating potassium current in rat neocortical pyramidal neurons”. In: *J Physiol* 581.3 (2007), pp. 941–960.

S6. A Korngreen and B Sakmann. “Voltage-gated K+ channels in layer 5 neocortical pyramidal neurones from young rats: subtypes and gradients”. In: *J Physiol* 525.3 (2000), pp. 621–639.

S7. AR Shepard and JL Rae. “Electrically silent potassium channel subunits from human lens epithelium”. In: *Am J Physiol-Cell Ph* 277.3 (1999), pp. C412–C424.

S8. JC Pineda, RS Waters, and RC Foehring. “Specificity in the interaction of HVA Ca2+ channel types with Ca2+-dependent AHPs and firing behavior in neocortical pyramidal neurons”. In: *J Neurophysiol* 79.5 (1998), pp. 2522–2534.

S9. SH Lee, TR DeCandia, S Ripke, J Yang, PF Sullivan, ME Goddard, MC Keller, et al. “Estimating the proportion of variation in susceptibility to schizophrenia captured by common SNPs”. In: *Nat Gen* 44.3 (2012), pp. 247–250.

S10. WA Catterall. “Structure and function of neuronal Ca2+ channels and their role in neurotransmitter release”. In: *Cell Calcium* 24.5 (1998), pp. 307–323.

S11. E Perez-Reyes. “Molecular physiology of low-voltage-activated t-type calcium channels”. In: *Physiol Rev* 83.1 (2003), pp. 117–161.

S12. HC Pape, T Munsch, and T Budde. “Novel vistas of calcium-mediated signalling in the thalamus”. In: *Pflugers Arch* 448.2 (2004), pp. 131–138.

S13. J Lee, K Song, K Lee, J Hong, H Lee, S Chae, E Cheong, et al. “Sleep spindles are generated in the absence of T-type calcium channel-mediated low-threshold burst firing of thalamocortical neurons”. In: *Proc Natl Acad Sci* 110.50 (2013), pp. 20266–20271.

S14. E Calixto, EJ Galván, JP Card, and G Barrionuevo. “Coincidence detection of convergent perforant path and mossy fibre inputs by CA3 interneurons”. In: *J Physiol* 586.11 (2008), pp. 2695–2712.

S15. D Ledergerber and ME Larkum. “The time window for generation of dendritic spikes by coincidence of action potentials and EPSPs is layer specific in somatosensory cortex”. In: *PLoS ONE* 7.3 (2012), e33146.

S16. M Kudrnac, S Beyl, A Hohaus, A Stary, T Peterbauer, E Timin, and S Hering. “Coupled and independent contributions of residues in IS6 and IIS6 to activation gating of CaV1.2”. In: *J Biol Chem* 284.18 (2009), pp. 12276–12284.

S17. JM Cordeiro, M Marieb, R Pfeiffer, K Calloe, E Burashnikov, and C Antzelevitch. “Accelerated inactivation of the L-type calcium current due to a mutation in CACNB2b underlies Brugada syndrome”. In: *J Mol Cell Cardiol* 46.5 (2009), pp. 695–703.

S18. E Massa, KM Kelly, DI Yule, RL MacDonald, and MD Uhler. “Comparison of fura-2 imaging and electrophysiological analysis of murine calcium channel alpha 1 subunits coexpressed with novel beta 2 subunit isoforms”. In: *Mol Pharmacol* 47.4 (1995), pp. 707–716.

S19. S Link, M Meissner, B Held, A Beck, P Weissgerber, M Freichel, and V Flockerzi. “Diversity and developmental expression of L-type calcium channel $\beta 2$ proteins and their influence on calcium current in murine heart”. In: *J Biol Chem* 284.44 (2009), pp. 30129–30137.

S20. BZ Tan, F Jiang, MY Tan, D Yu, H Huang, Y Shen, and TW Soong. “Functional characterization of alternative splicing in the C terminus of L-type CaV1. 3 channels”. In: *J Biol Chem* 286.49 (2011), pp. 42725–42735.

S21. G Bock, M Gebhart, A Scharinger, W Jangsangthong, P Busquet, C Poggiani, S Sartori, et al. “Functional properties of a newly identified C-terminal splice variant of Cav1. 3 L-type Ca2+ channels”. In: *J Biol Chem* 286.49 (2011), pp. 42736–42748.

S22. Q Zhang, V Timofeyev, H Qiu, L Lu, N Li, A Singapuri, CL Torado, et al. “Expression and roles of Cav1.3 ($\alpha$1D) L-type Ca2+ channel in atrioventricular node automaticity”. In: *J Mol Cell Cardiol* 50.1 (2011), pp. 194–202.

S23. A Pérez-Alvarez, A Hernández-Vivanco, JC Caba-González, and A Albillos. “Different roles attributed to Cav1 channel subtypes in spontaneous action potential firing and fine tuning of exocytosis in mouse chromaffin cells”. In: *J Neurochem* 116.1 (2011), pp. 105–121.

S24. J Murbartián, JM Arias, and E Perez-Reyes. “Functional impact of alternative splicing of human T-type Cav3.3 calcium channels”. In: *J Neurophysiol* 92.6 (2004), pp. 3399–3407.

S25. Y Ji, MJ Lalli, GJ Babu, Y Xu, DL Kirkpatrick, LH Liu, N Chiamvimonvat, et al. “Disruption of a single copy of the SERCA2 gene results in altered Ca2+ homeostasis and cardiomyocyte function”. In: *J Biol Chem* 275.48 (2000), pp. 38073–38080.

S26. AK Fakira, LD Gaspers, AP Thomas, H Li, MR Jain, and S Elkabes. “Purkinje cell dysfunction and delayed death in plasma membrane calcium ATPase 2-heterozygous mice”. In: *Mol Cell Neurosci* 51.1 (2012), pp. 22–31.

S27. RM Empson, W Akemann, and T Knöpfel. “The role of the calcium transporter protein plasma membrane calcium ATPase PMCA2 in cerebellar Purkinje neuron function”. In: *Funct Neurol* 25.3 (2010), p. 153.

S28. R Ficarella, F Di Leva, M Bortolozzi, S Ortolano, F Donaudy, M Petrillo, S Melchionda, et al. “A functional study of plasma-membrane calcium-pump isoform 2 mutants causing digenic deafness”. In: *Proc Natl Acad Sci* 104.5 (2007), pp. 1516–1521.

S29. S Cestèle, P Scalmani, R Rusconi, B Terragni, S Franceschetti, and M Mantegazza. “Self-limited hyperexcitability: Functional effect of a familial hemiplegic migraine mutation of the Nav1.1 (SCN1A) Na+ channel”. In: *J Neurosci* 28.29 (2008), pp. 7273–7283.

S30. KR Vanmolkot, E Babini, B de Vries, AH Stam, T Freilinger, GM Terwindt, L Norris, et al. “The novel p.L1649Q mutation in the SCN1A epilepsy gene is associated with familial hemiplegic migraine: genetic and functional studies”. In: *Hum Mutat* 28.5 (2007), pp. 522–522.

S31. M Estacion, C Han, JS Choi, J Hoeijmakers, G Lauria, J Drenth, MM Gerrits, et al. “Intra- and interfamily phenotypic diversity in pain syndromes associated with a gain-of-function variant of NaV1.7”. In: *Mol Pain* 7 (2011), p. 92.

S32. M Estacion, S Dib-Hajj, P Benke, RH te Morsche, E Eastman, L Macala, J Drenth, et al. “NaV1.7 gain-of-function mutations as a continuum: A1632E displays physiological changes associated with erythromelalgia and paroxysmal extreme pain disorder mutations and produces symptoms of both disorders”. In: *J Neurosci* 28.43 (2008), pp. 11079–11088.

S33. C Han, AM Rush, SD Dib-Hajj, S Li, Z Xu, Y Wang, L Tyrrell, et al. “Sporadic onset of erythermalgia: A gain-of-function mutation in Nav1.7”. In: *Ann Neurol* 59.3 (2006), pp. 553–558.

S34. S Dib-Hajj, A Rush, T Cummins, F Hisama, S Novella, L Tyrrell, L Marshall, et al. “Gain-of-function mutation in Nav1.7 in familial erythromelalgia induces bursting of sensory neurons”. In: *Brain* 128.8 (2005), pp. 1847–1854.

S35. E Bocksteins, N Ottschytsch, JP Timmermans, A Labro, and D Snyders. “Functional interactions between residues in the S1, S4, and S5 domains of Kv2.1”. In: *Eur Biophys J* 40.6 (2011), pp. 783–793.

S36. OH Wittekindt, V Visan, H Tomita, F Imtiaz, JJ Gargus, F Lehmann-Horn, S Grissmer, et al. “An apamin-and scyllatoxin-insensitive isoform of the human SK3 channel”. In: *Mol Pharmacol* 65.3 (2004), pp. 788–801.

S37. TM Ishii, N Nakashima, and H Ohmori. “Tryptophan-scanning mutagenesis in the S1 domain of mammalian HCN channel reveals residues critical for voltage-gated activation”. In: *J Physiol* 579.2 (2007), pp. 291–301.

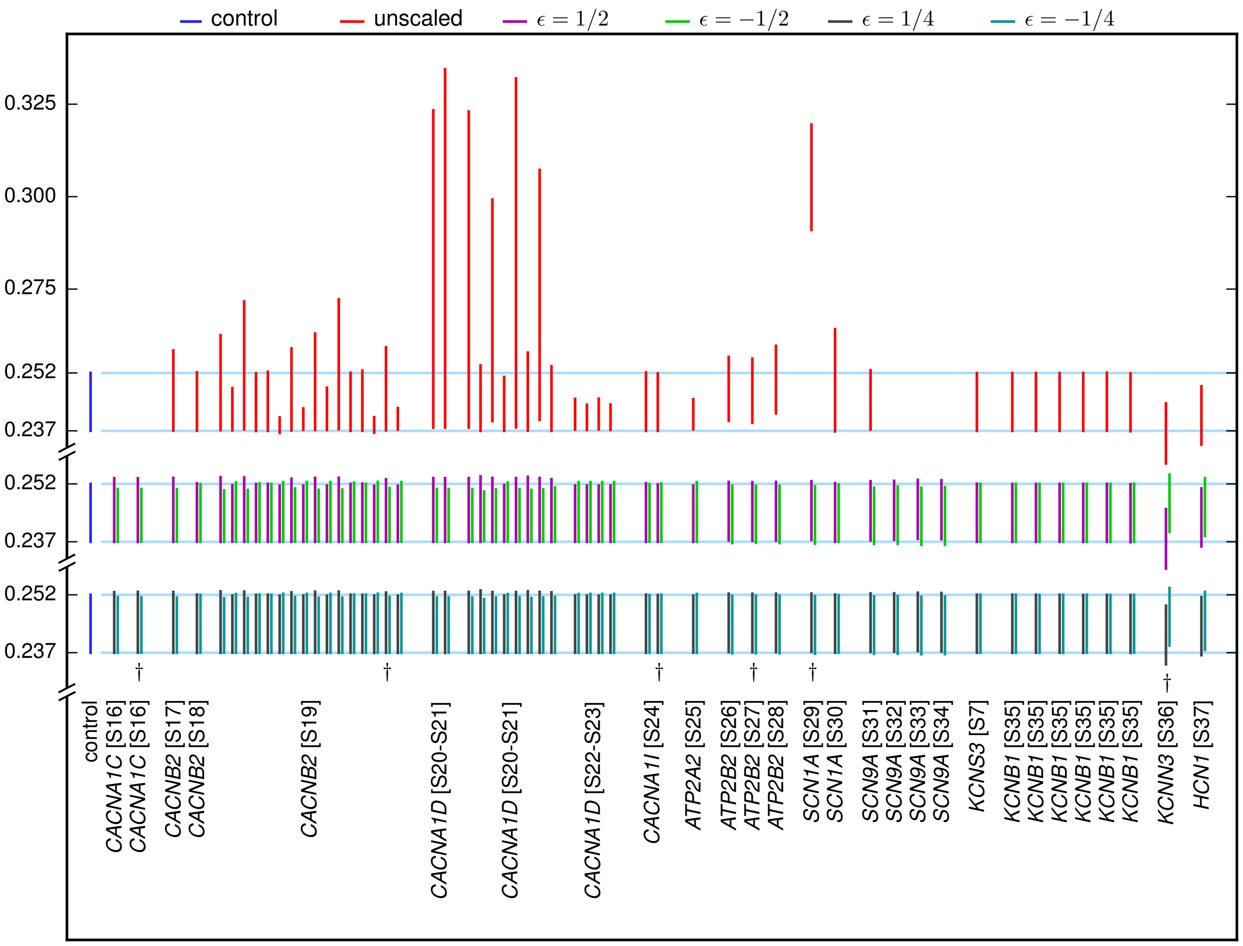


Figure S1: **Ranges of $Ca^{2+}$ concentration in simulations of steady-state firing in cells with different genetic variants implemented**. The blue bars (and the light blue horizontal lines) show the minimum and maximum $Ca^{2+}$ concentration as a response to a 1.2 nA DC injection in a control neuron, while the other colors show the corresponding quantities in neurons with the variants from Table 2 implemented. The red bars in the upper plot show the effects of the unscaled variants, while the bars in the middle plot show the effects of the $\epsilon = \frac{1}{2}$ (magenta) and $\epsilon = -\frac{1}{2}$ (green) downscaled variants. The bars in the lower plot show the effect of minimally scaled (dark gray: $\epsilon = \frac{1}{4}$, cyan: $\epsilon = -\frac{1}{4}$) variants. The missing red bars among *CACNA1C* and *SCN9A* variants represent cases where the unscaled variant expresses large depolarization even without an input, and the membrane potential repolarization is missing or too weak to maintain the spiking behavior. The variants are based on previous experimental studies [S7, S16–S37] and they are ordered as in Table 2. The variants marked with † were used in Figures 2–6.

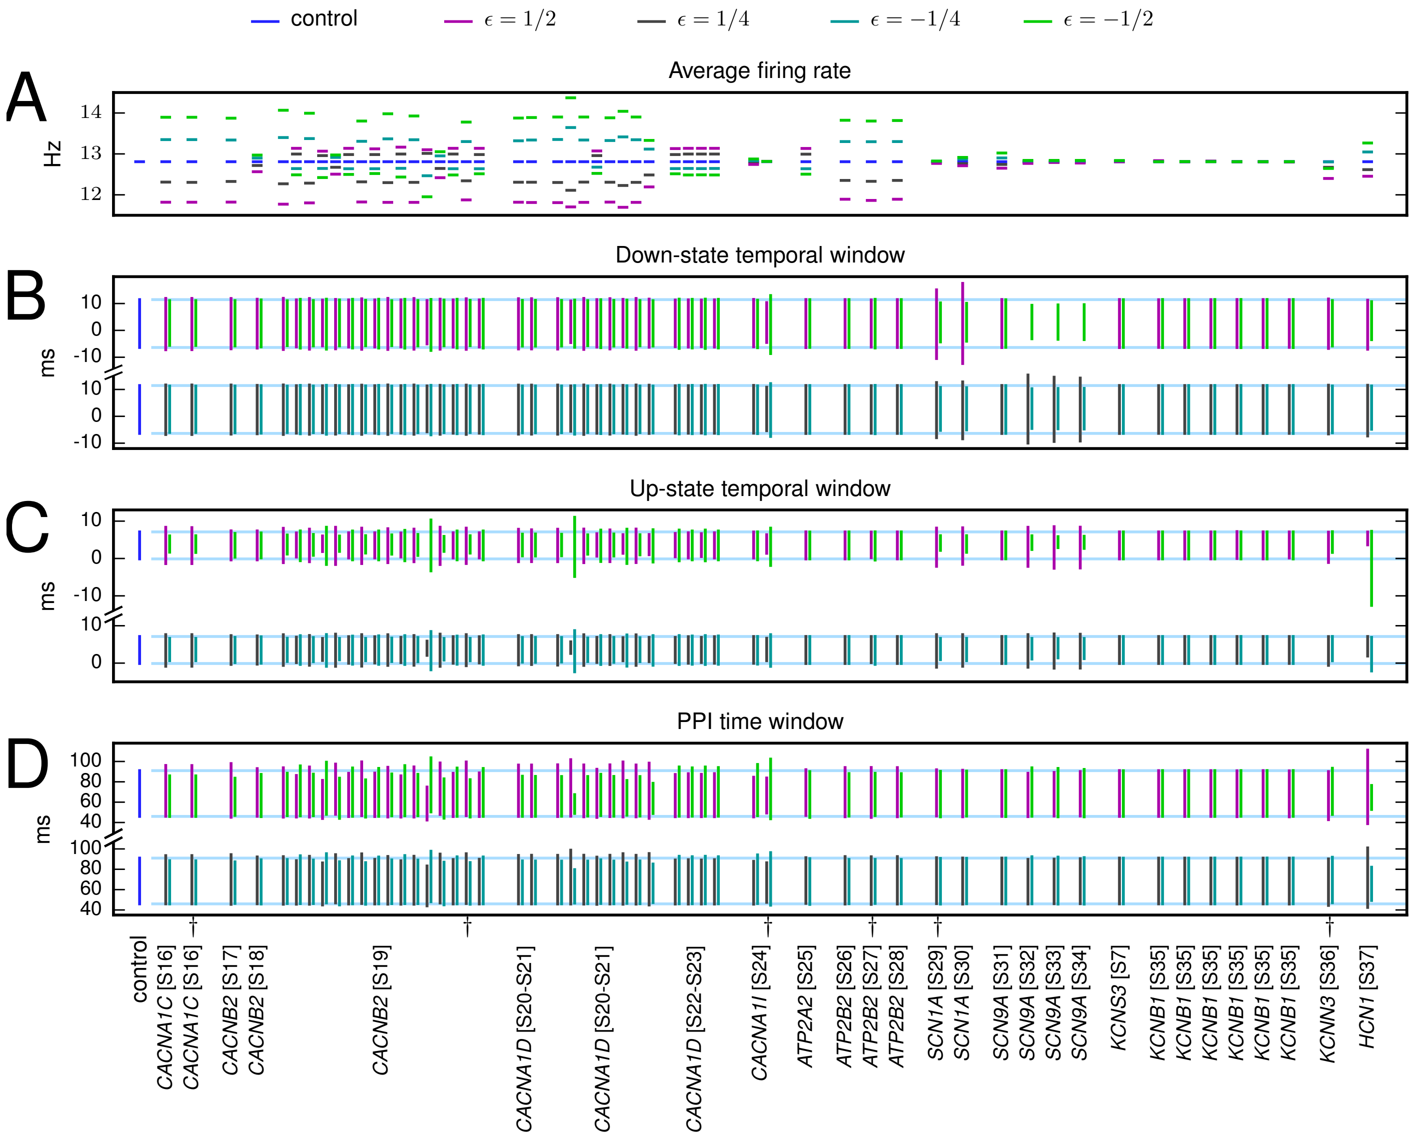


Figure S2: **Various statistics from neurons with different downscaled genetic variants implemented**. **A**: The average steady-state spiking frequency (see Figure 3) when a somatic DC of amplitude 0.35–1.4 nA was injected. Data plotted for each variant in Table 2. **B**: The down-state temporal window span (see Figure 5). The plotted range corresponds to the range of ISIs for which the maximum membrane potential at the apical dendrite was larger than -14.05 mV (the midpoint between the highest and lowest apical dendrite membrane potentials across all ISIs for the control neuron). **C**: The up-state temporal window span (see Figure 5) of ISIs that produced a peak apical dendrite membrane potential larger than -23.21 mV, illustrated in a similar manner as in panel B. **D**: The temporal window for large single-cell prepulse inhibition (PPI, see Figure 6). The plotted ranges correspond to the ISIs for which a larger than three-fold second apical stimulus was required to induce an extra spike. In all panels, the blue bars (and the light blue horizontal lines) correspond to the control neuron values, while the magenta and green bars correspond to the $\epsilon = \frac{1}{2}$ (magenta) and $\epsilon = -\frac{1}{2}$ (green) downscaled variants, and the dark gray and cyan bars correspond to the $\epsilon = \frac{1}{4}$ (dark gray) and $\epsilon = -\frac{1}{4}$ (cyan) downscaled variants. The missing bars in panel B among *SCN9A* variants correspond to cases where the somatic pulse alone was sufficient to produce a large $Ca^{2+}$ spike (apical dendrite membrane potential larger than -14.05 mV). The missing bars in panel C among *CACNB2* and *CACNA1D* variants correspond to cases where no ISI produced a large $Ca^{2+}$ spike (i.e., the apical dendrite membrane potential always remained smaller than -23.21 mV). The variants marked with † were used in Figures 2–6.

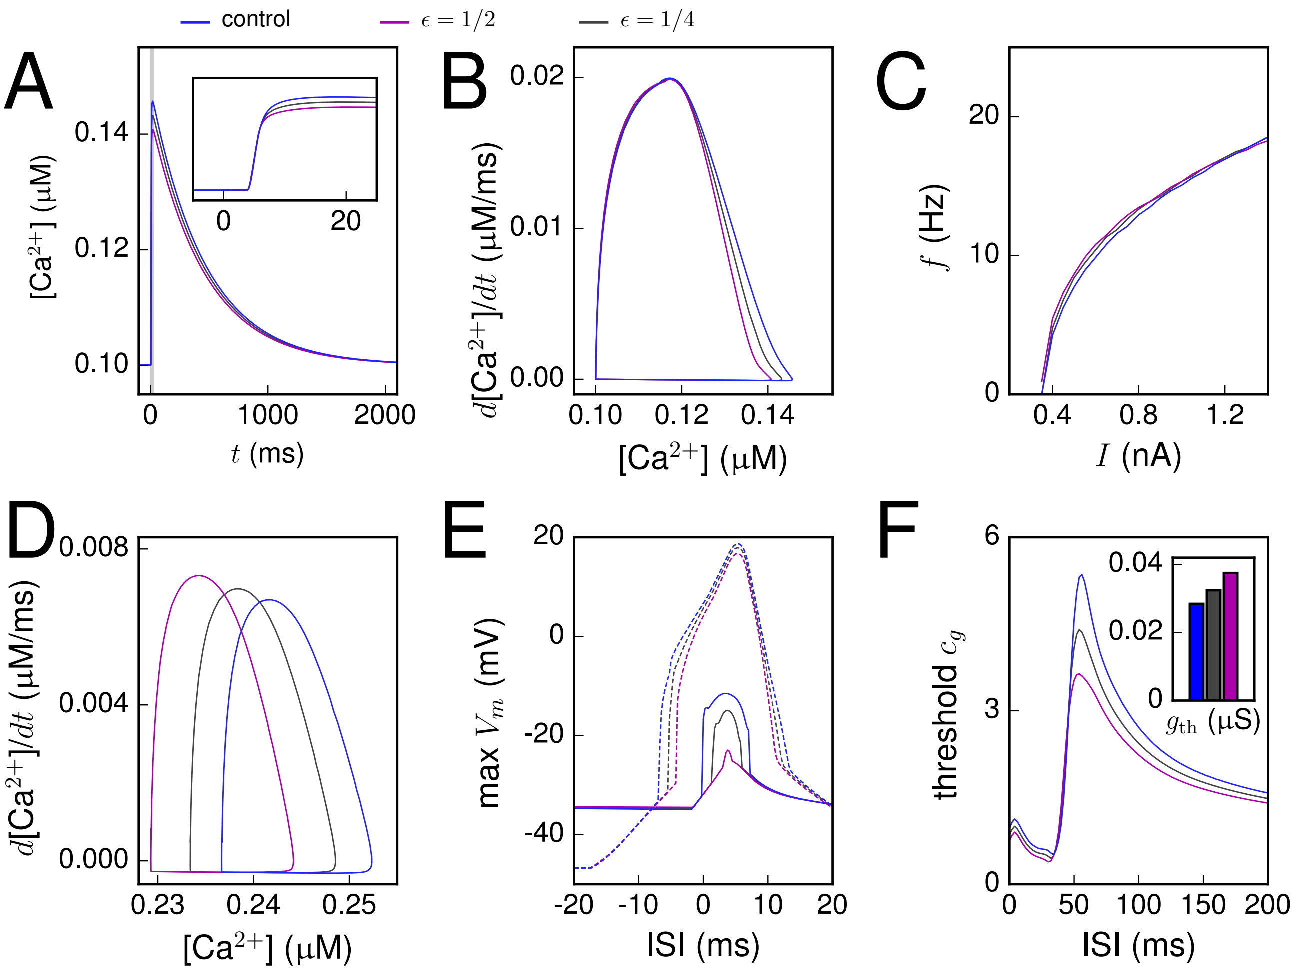


Figure S3: **Combined genetic variants can radically change the neuron response.** A combination of six downscaled variants from Table 2 (*CACNB2* [S19], *CACNA1D* [S22, S23], *CACNA1I* [S24], *ATP2A2* [S25], and *KCNN3* [S36]) was applied. These variants were chosen as an example combination as they all showed weakened prepulse inhibition (see Figure 6). The gray curves show the properties of a neuron with the combination of $\epsilon = \frac{1}{4}$ downscaled variants, and the magenta curves represent the combination of $\epsilon = \frac{1}{2}$ downscaled variants. **A-B**: [Ca$^{2+}$] response to short somatic stimulus, shown in time series (A) and phase plane (B). See Figure 2B and 2C for details. **C**: f-I curves. See Figure 3 for details. **D**: [Ca$^{2+}$] response to prolonged stimulus. See Figure 4 for details. **E**: Integration of apical and somatic stimulus during up and down states. See Figure 5 for details. The combination of $\epsilon = \frac{1}{2}$ variants did not respond with a strong $Ca^{2+}$ spike for any inter-stimulus interval. **F**: Threshold conductance factor for a second spike. See Figure 6 for details. A strong second stimulus with four-fold total conductance with respect to the threshold conductance would always make the neuron with combined $\epsilon = \frac{1}{2}$ variants spike, while the neuron with combined $\epsilon = \frac{1}{4}$ variants would inhibit it for ISI$\in$[49 ms, 61 ms], and the control neuron would inhibit it for ISI$\in$[49 ms, 71 ms].

Table S2: **Effects of positively scaled variants on steady-state firing, integration of somatic and apical inputs, and inhibition of a second apical stimulus**. The shown effects are extracted from the properties of the $\epsilon = \frac{1}{2}$ variant in Figure S2. The variants are ordered as in Table 2, and the first column shows the name of the underlying gene. The second column shows whether the average firing rate (see Figure S2A) of the variant is increased ('+') or decreased ('–') with respect to the control neuron. A "minuscule" effect refers to cases where the effect was smaller than 0.5% of the control neuron average firing rate. The third and fourth columns show how the down and up-state windows (see Figure S2B–C) are affected in the variant. A "broader" window refers to an effect where the variant window starts at an ISI smaller than the start of the control window and ends at an ISI greater than the end of the control window. By contrast, in a "narrower" case the window starts at an ISI greater than the start of the control window and ends at a smaller ISI than the end of the control window. If both the starting point and end point of the window are moved to the same direction with respect to the control window, the table entry is "moved forward" (toward smaller ISIs) or "delayed" (toward larger ISIs). Cases where both end points moved less than 5% of the width of the temporal window in a control neuron are labeled as "minuscule" effects, regardless the direction to which the end points moved. Finally, the value "N/A" denotes cases where the temporal window could not be defined. The fifth column shows the corresponding properties for the PPI window (see Figure S2D). The variants marked with † are the ones that were used in Figures 2–6. The horizontal lines separate variants that are based on different sets of experimental data, see Table 1.

| Gene | f-I curve average | Down-state window | Up-state window | PPI window | |
|---|---|---|---|---|---|
| *CACNA1C* | – | Minuscule | Broader | Delayed | |
| *CACNA1C* | – | Minuscule | Broader | Delayed | † |
| *CACNB2* | – | Minuscule | Minuscule | Broader | |
| *CACNB2* | – | Minuscule | Minuscule | Minuscule | |
| *CACNB2* | – | Minuscule | Broader | Broader | |
| *CACNB2* | + | Minuscule | Narrower | Moved forward | |
| *CACNB2* | – | Minuscule | Broader | Broader | |
| *CACNB2* | + | Minuscule | Narrower | Moved forward | |
| *CACNB2* | – | Minuscule | Broader | Delayed | |
| *CACNB2* | + | Minuscule | Minuscule | Moved forward | |
| *CACNB2* | – | Minuscule | Broader | Delayed | |
| *CACNB2* | + | Minuscule | Minuscule | Moved forward | |
| *CACNB2* | – | Minuscule | Broader | Broader | |
| *CACNB2* | + | Minuscule | Narrower | Moved forward | |
| *CACNB2* | – | Minuscule | Broader | Broader | |
| *CACNB2* | + | Narrower | N/A | Moved forward | |
| *CACNB2* | – | Minuscule | Broader | Delayed | |
| *CACNB2* | + | Minuscule | Minuscule | Moved forward | |
| *CACNB2* | – | Minuscule | Broader | Delayed | † |
| *CACNB2* | + | Minuscule | Minuscule | Minuscule | |
| *CACNA1D* | – | Minuscule | Broader | Delayed | |
| *CACNA1D* | – | Minuscule | Broader | Broader | |
| *CACNA1D* | – | Minuscule | Broader | Broader | |
| *CACNA1D* | – | Narrower | N/A | Delayed | |
| *CACNA1D* | – | Minuscule | Broader | Broader | |
| *CACNA1D* | + | Minuscule | Narrower | Minuscule | |
| *CACNA1D* | – | Minuscule | Broader | Broader | |
| *CACNA1D* | – | Minuscule | Narrower | Broader | |
| *CACNA1D* | – | Minuscule | Broader | Broader | |
| *CACNA1D* | – | Minuscule | Narrower | Broader | |
| *CACNA1D* | + | Minuscule | Narrower | Moved forward | |
| *CACNA1D* | + | Minuscule | Minuscule | Moved forward | |
| *CACNA1D* | + | Minuscule | Narrower | Moved forward | |
| *CACNA1D* | + | Minuscule | Minuscule | Moved forward | |
| *CACNA1I* | – | Minuscule | Minuscule | Moved forward | |
| *CACNA1I* | Minuscule | Narrower | Narrower | Narrower | † |
| *ATP2A2* | + | Minuscule | Minuscule | Minuscule | |
| *ATP2B2* | – | Minuscule | Minuscule | Broader | |
| *ATP2B2* | – | Minuscule | Minuscule | Broader | † |
| *ATP2B2* | – | Minuscule | Minuscule | Broader | |
| *SCN1A* | Minuscule | Broader | Broader | Minuscule | † |
| *SCN1A* | – | Broader | Broader | Minuscule | |
| *SCN9A* | – | Minuscule | Minuscule | Minuscule | |
| *SCN9A* | Minuscule | N/A | Broader | Moved forward | |
| *SCN9A* | Minuscule | N/A | Broader | Minuscule | |
| *SCN9A* | Minuscule | N/A | Broader | Minuscule | |
| *KCNS3* | No change | Minuscule | Minuscule | Minuscule | |
| *KCNB1* | Minuscule | Minuscule | Minuscule | Minuscule | |
| *KCNB1* | No change | Minuscule | Minuscule | Minuscule | |
| *KCNB1* | Minuscule | Minuscule | Minuscule | Minuscule | |
| *KCNB1* | No change | Minuscule | Minuscule | Minuscule | |
| *KCNB1* | No change | Minuscule | Minuscule | Minuscule | |
| *KCNB1* | Minuscule | Minuscule | Minuscule | Minuscule | |
| *KCNN3* | – | Minuscule | Moved forward | Moved forward | † |
| *HCN1* | – | Minuscule | Narrower | Broader | |

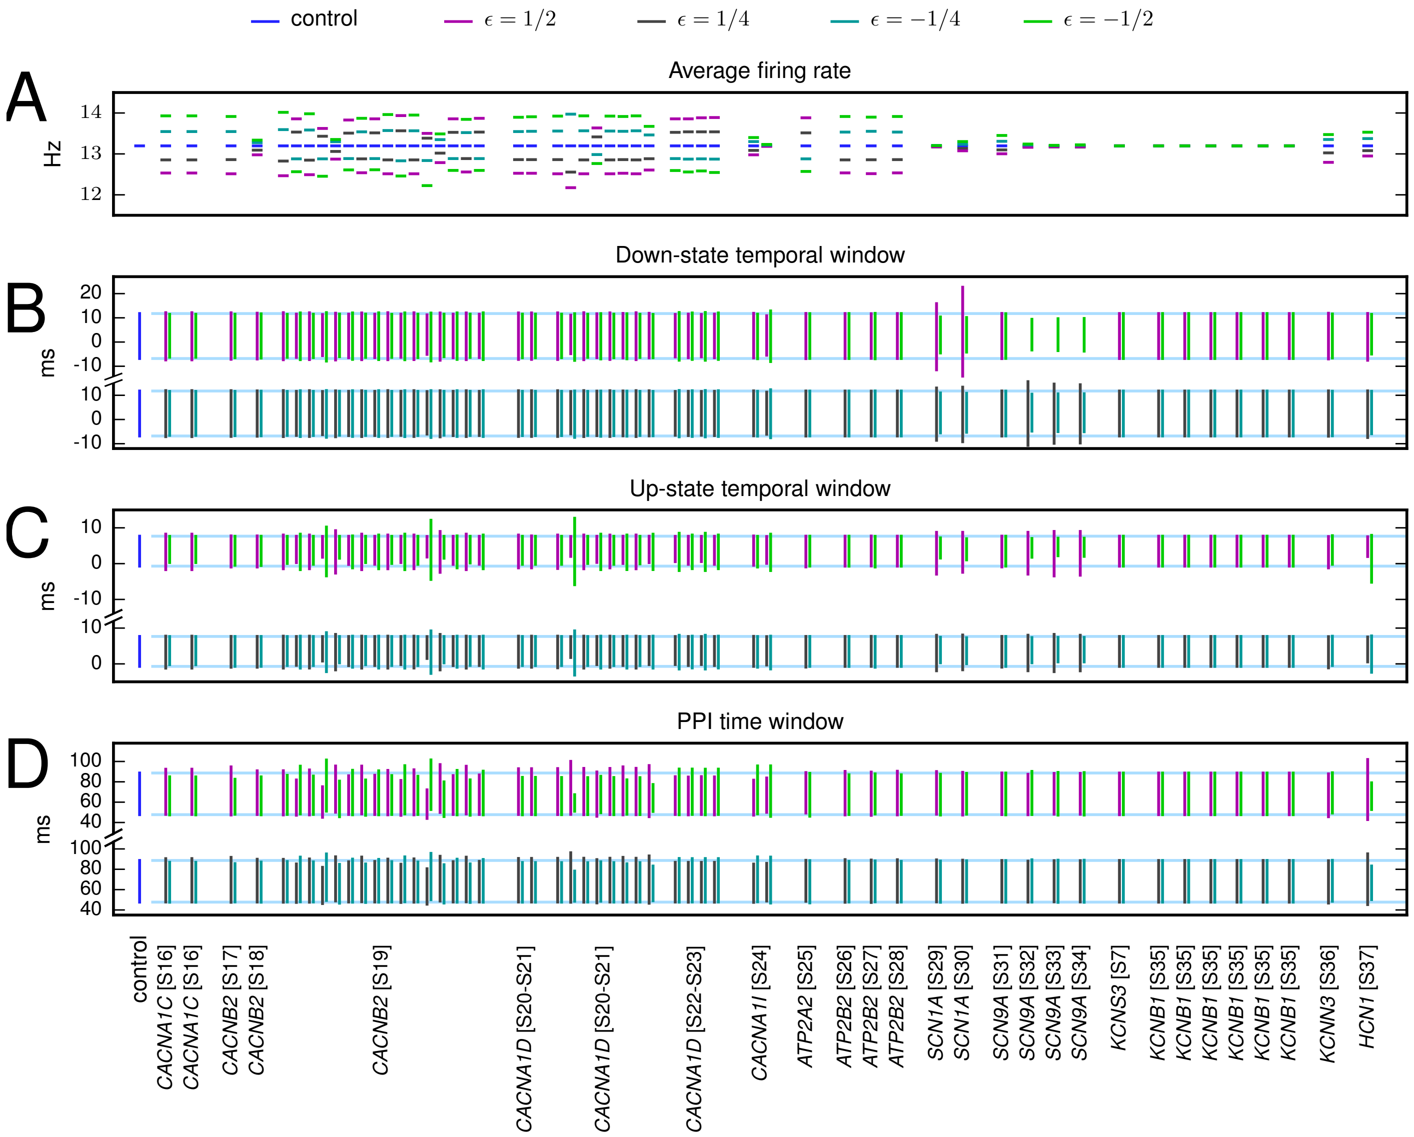


Figure S4: **Various statistics from neurons with alternative set of fitted model parameters and different downscaled genetic variants implemented**. The maximal conductances and parameters controlling $Ca^{2+}$ dynamics from Table S1 in [S2] ("Model 1") were applied, while other parameters were kept fixed. **A**: The average steady-state spiking frequency when a somatic DC of amplitude 0.35–1.4 nA was injected. See Figure S2A for the corresponding results in the neuron model with default parameters. **B**: The down-state temporal window span. See Figure S2B. **C**: The up-state temporal window span. See Figure S2C. **D**: The temporal window for large single-cell prepulse inhibition. See Figure S2D.

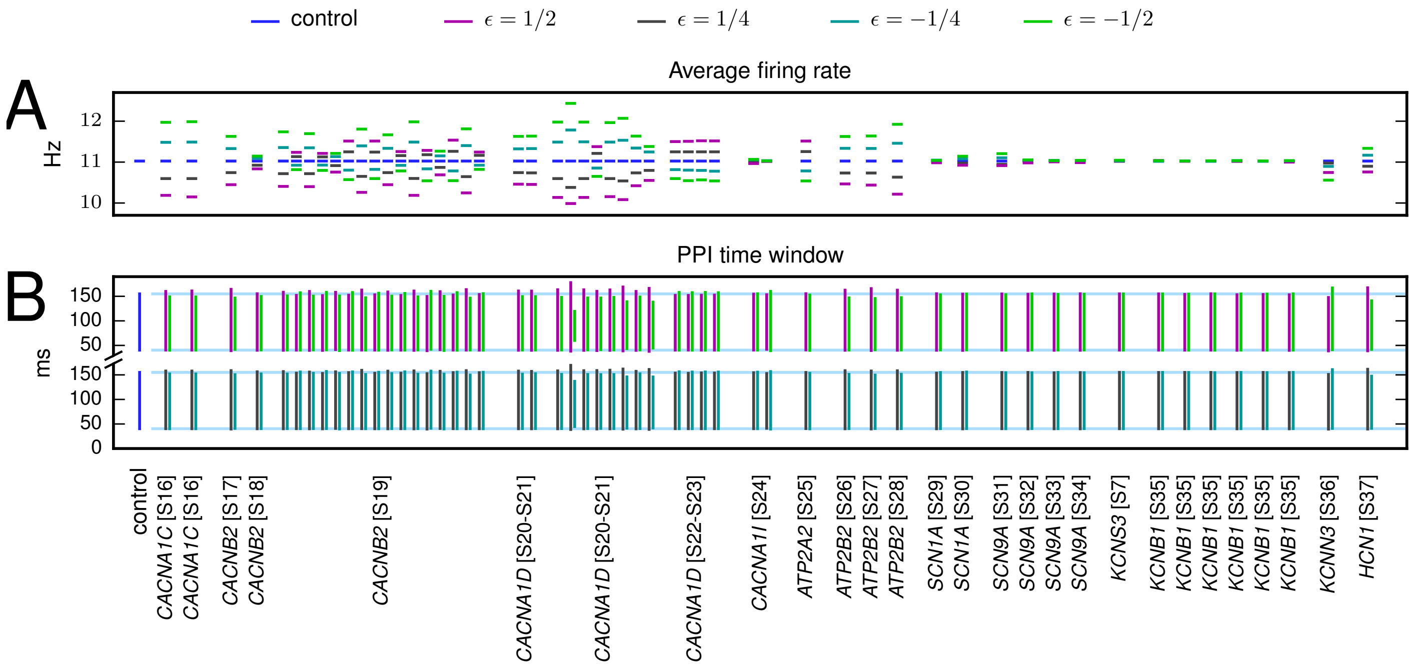


Figure S5: **Average firing frequency and PPI statistics from neurons with alternative morphology and different downscaled genetic variants implemented**. The cell morphology #2 of [S2] was used with the default model parameters. **A**: The average steady-state spiking frequency when a somatic DC of amplitude 0.35–1.4 nA was injected. See Figure S2A for the corresponding results in cell #1. **B**: The temporal window for large single-cell prepulse inhibition. See Figure S2D. The plotted ranges correspond to the ISIs for which a larger than 1.5-fold second apical stimulus was required to induce an extra spike.
